# Supplementary material for: Disadvantaged Communities Have Lower Access to Urban Infrastructure
Source: arXiv:2203.13784 ancillary file (2022-03-25)
Supplement: Supplementary file 1 [file 2022_Nicoletti_Accessibility_SciAdvances_SI.pdf]

# Supplementary Information: Disadvantaged Communities Have Lower Access to Urban Infrastructure

Leonardo Nicoletti[1*], Mikhail Sirenko[1], Trivik Verma[1]

[1]Faculty of Technology, Policy and Management,
Delft University of Technology, 2628BX Delft, The Netherlands

[*]To whom correspondence should be addressed; E-mail: t.verma@tudelft.nl

March 25, 2022

# 1 Distributions of Accessibility

## 1.1 Log-normal Distributions

Looking at the histograms of accessibility, visually, we can infer that that the accessibility score $A \in [0, 1]$ for the spatial units of any given city is either normally distributed (a log-normal distribution: accessibility is calculated using a log function of distances) or a mixture of multiple normal distributions 1. To qualify this observation, we apply the Shapiro-Wilk normality test to each of the 54 cities of interest. Our choice for the Shapiro-Wilk test is driven by the fact that it has proven to have a higher *power* (the probability of a hypothesis test that a potential effect is detected) than, for example, Kolmogorov-Smirnov (*1*). However, normality tests, including Shapiro-Wilk one, are sensitive to the sample size. That is, given a large enough sample, the null hypothesis (the sample is normally distributed) will always be rejected. Thus, we cannot simply take a random sample from the population: accessibility in many cities is skewed or has long tails (see statistical reporting in Table 1). We run the test 100,000 times (trials) on different subsets of 250 observations (sampling without replacement) from the original sample to overcome these issues. Next, we count the number of times the *p*-value is less than $\alpha = 0.05$ (the null hypothesis is accepted) for each city. To decide whether the data is normally distributed, we use a threshold parameter called *Acceptance Rate (AR)*, in 50%: if in 50,000 out of 100,000 times the null hypothesis was accepted, we assume that the data is ”close enough” to

be normally distributed. The acceptance rate is equal to the number of times the null hypothesis was accepted divided by the total number of trials. It is critical to mention that we do not aim to identify the ”true” distribution (normal) of the data by applying such a procedure. Instead, we seek to determine which cities exhibit accessibility distributions that are ”close enough” to a normal distribution.

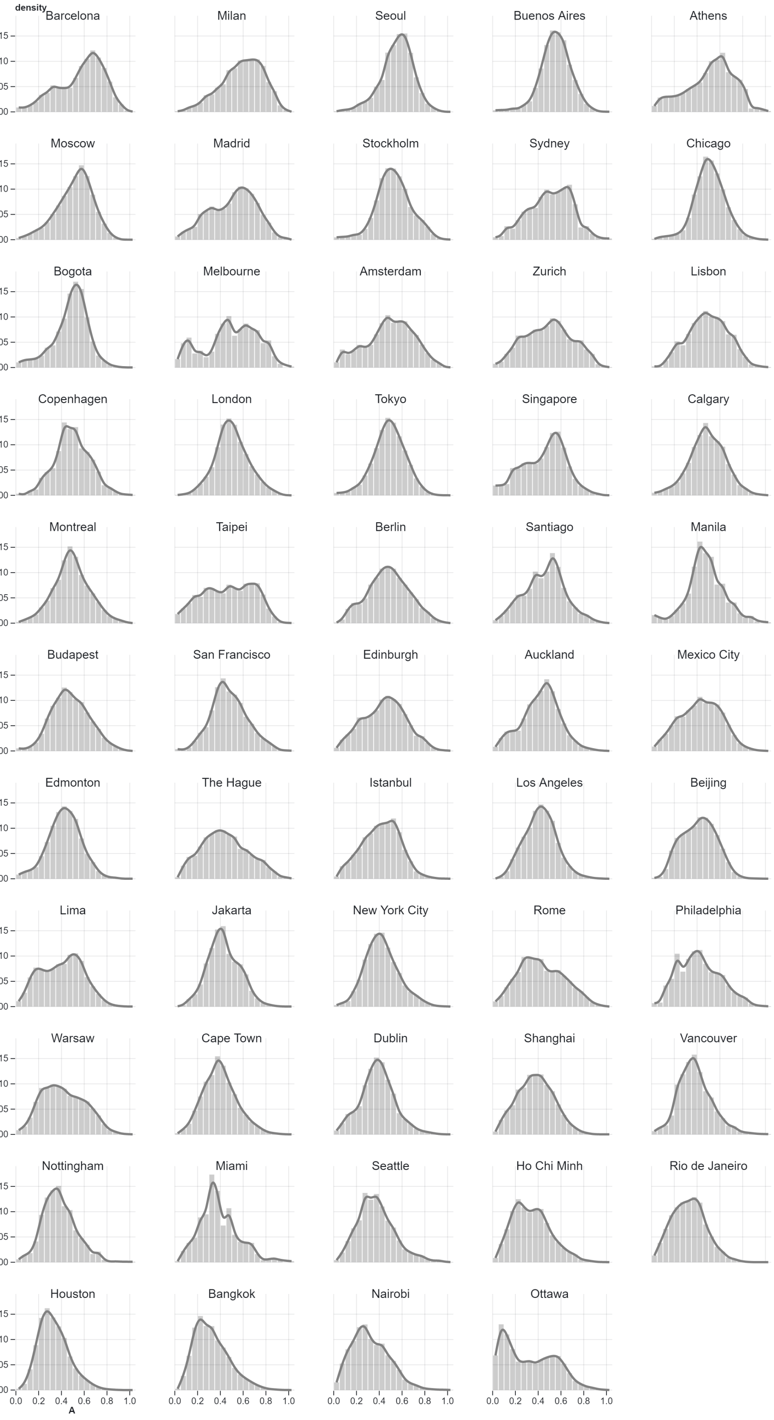


Supplementary Fig. 1: Statistical distribution of accessibility for all 54 cities showing log-normal or mixed distributions.

Supplementary Table 1: Statistical information of Accessibility (A) Distributions of the 54 cities. The columns show the count of Points of interest (POIs) and spatial units, spatial density of points and median of A. The min and max values of A are always 0 and 1, respectively, as the scores are normalised and comparing them would be meaningless across cities due to the difference in their land areas. Number of Points of interest (POIs) were collected for each city using the OsmNX Python package (*2*) and the spatial units are obtained from the GHSL data base (*3*). Each of the 10 cities in the subset analysis of socioeconomic variables is indicated in **bold**.

| City | POIs Collected | Spatial Units | Point Density | Median (A) | Standard Deviation (A) |
|---|---|---|---|---|---|
| Amsterdam | 34767 | 2365 | 14,7 | 0.51 | 0.21 |
| Athens | 14584 | 599 | 24,35 | 0.55 | 0.21 |
| Auckland | 74903 | 10495 | 7,14 | 0.44 | 0.16 |
| Bangkok | 108127 | 14872 | 7,27 | 0.30 | 0.15 |
| Barcelona | 26362 | 1489 | 17,7 | 0.61 | 0.20 |
| Beijing | 41426 | 10232 | 4,05 | 0.42 | 0.15 |
| Berlin | 164610 | 12492 | 13,18 | 0.48 | 0.18 |
| Bogota | 91215 | 6298 | 14,48 | 0.51 | 0.15 |
| Budapest | 77464 | 7314 | 10,59 | 0.47 | 0.16 |
| Buenos Aires | 29370 | 3162 | 9,29 | 0.55 | 0.13 |
| Calgary | 94697 | 8755 | 10,82 | 0.49 | 0.16 |
| Cape Town | 106271 | 12816 | 8,29 | 0.39 | 0.15 |
| **Chicago** | 107285 | 8455 | 12,69 | 0.51 | 0.13 |
| Copenhagen | 23289 | 1304 | 17,86 | 0.49 | 0.15 |
| Dublin | 78088 | 6538 | 11,94 | 0.38 | 0.15 |
| Edinburgh | 33109 | 2431 | 13,62 | 0.46 | 0.18 |
| Edmonton | 53924 | 6735 | 8,01 | 0.43 | 0.15 |
| Ho Chi Minh | 97760 | 9602 | 10,18 | 0.33 | 0.16 |
| **Houston** | 251804 | 31661 | 7,95 | 0.32 | 0.13 |
| Istanbul | 172385 | 16171 | 10,66 | 0.42 | 0.16 |
| Jakarta | 128741 | 9750 | 13,2 | 0.42 | 0.14 |
| Lima | 148190 | 12144 | 12,2 | 0.42 | 0.18 |
| Lisbon | 23816 | 1297 | 18,36 | 0.50 | 0.17 |
| London | 249061 | 21772 | 11,44 | 0.49 | 0.14 |
| **Los Angeles** | 121797 | 15335 | 7,94 | 0.42 | 0.14 |
| Madrid | 94012 | 5194 | 18,1 | 0.54 | 0.20 |
| Manila | 7306 | 564 | 12,95 | 0.47 | 0.16 |
| Melbourne | 12212 | 541 | 22,57 | 0.51 | 0.23 |
| Mexico City | 111559 | 12257 | 9,1 | 0.44 | 0.18 |
| **Miami** | 1239 | 496 | 2,5 | 0.36 | 0.17 |
| Milan | 44188 | 2401 | 18,4 | 0.61 | 0.18 |
| **Montreal** | 166189 | 6431 | 25,84 | 0.49 | 0.16 |
| Moscow | 300904 | 14560 | 20,67 | 0.54 | 0.16 |
| Nairobi | 31317 | 5632 | 5,56 | 0.30 | 0.16 |
| **New York City** | 127029 | 11166 | 11,38 | 0.41 | 0.15 |
| Nottingham | 21587 | 1047 | 20,62 | 0.37 | 0.14 |
| Ottawa | 181581 | 12015 | 15,11 | 0.30 | 0.22 |
| **Philadelphia** | 7989 | 1635 | 4,89 | 0.40 | 0.18 |
| Rio de Janeiro | 68084 | 9992 | 6,81 | 0.33 | 0.15 |
| Rome | 75468 | 9002 | 8,38 | 0.41 | 0.20 |
| **San Francisco** | 30676 | 1895 | 16,19 | 0.46 | 0.16 |
| Santiago | 53343 | 4640 | 11,5 | 0.47 | 0.18 |
| **Seattle** | 74767 | 3355 | 22,29 | 0.36 | 0.16 |
| Seoul | 95824 | 7586 | 12,63 | 0.57 | 0.14 |
| Shanghai | 29916 | 7136 | 4,19 | 0.37 | 0.16 |
| Singapore | 81377 | 7040 | 11,56 | 0.49 | 0.19 |
| Stockholm | 41703 | 3001 | 13,9 | 0.52 | 0.15 |
| Sydney | 8019 | 414 | 19,37 | 0.52 | 0.19 |
| Taipei | 46735 | 3270 | 14,29 | 0.48 | 0.22 |
| The Hague | 23924 | 1319 | 18,14 | 0.43 | 0.20 |
| Tokyo | 393431 | 20094 | 19,58 | 0.49 | 0.14 |
| **Vancouver** | 138770 | 1850 | 75,01 | 0.37 | 0.15 |
| Warsaw | 127647 | 6884 | 18,54 | 0.40 | 0.18 |
| Zurich | 32994 | 1377 | 23,96 | 0.50 | 0.21 |

We found that 17 out of 54 cities are above the threshold. Figure 2 presents log accessibility histograms along with the KDEs for this subset. For some cities like Copenhagen or Montreal, such an approach works: the mean is centred around 0.5 with more or less equally sized left and right tail. However, accessibility for Berlin, Santiago, Jakarta and Dublin seem to be composed of more than one normal distribution. We added them to other 37 cities for which the hypothesis was rejected (see statistical reporting in Table 2).

Visual inspection of Figure 3 indicates three potential causes for rejection of the null hypothesis: skewness (e.g. Seoul), mixture distribution (e.g. Ottawa), long(-er) or asymmetric tails (e.g. Stockholm).

As the next step, we apply a Gaussian mixture model (GMM) (*4,5*) to the 41 cities for which we established that the null hypothesis is rejected. GMM can be used as a clustering algorithm to find the number of normal distributions in the data and their parameters. Our approach here is two-fold. Since GMM is a type of unsupervised learning algorithm, the ”true” cluster labels and the number of clusters are unknown. Therefore, we first search for the number of clusters that has the highest Silhouette Coefficient (SC) (*6*). Silhouette Coefficient is a metric to evaluate clustering quality when the true labels are unknown. Second, we use the number of clusters to build and fit the GMM model to the data. Figures 4 and 5 show the results of fitting GMM to the data.

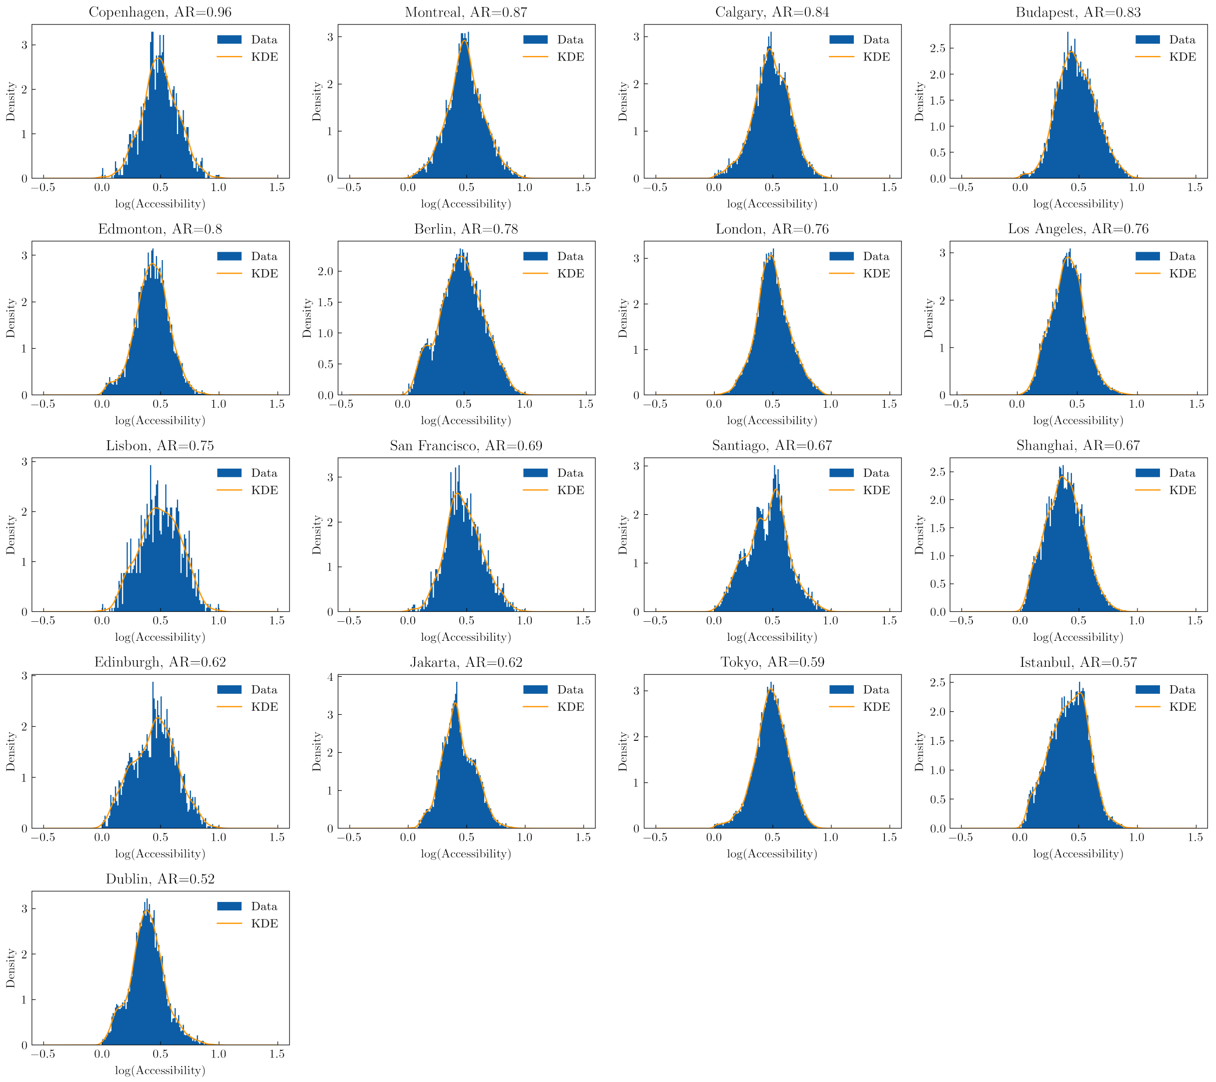


Supplementary Fig. 2: Accessibility distributions of cities showing histograms and kernel density plots for those where Acceptance Rate (AR) $\geq .5$.

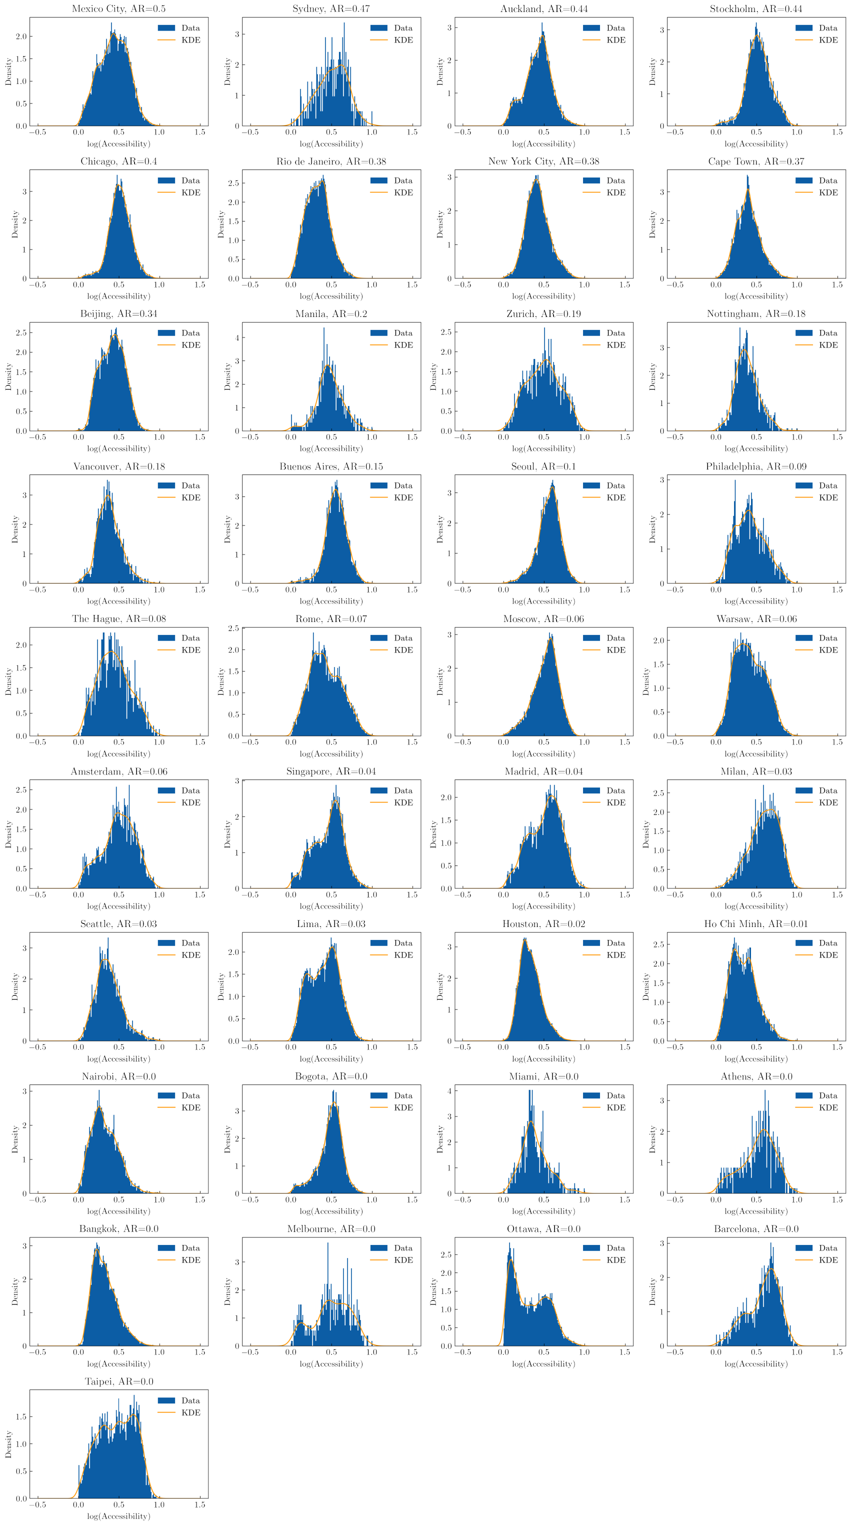


Supplementary Fig. 3: Accessibility distributions of cities showing histograms and kernel density plots for those where Acceptance Rate (AR) $< .5$. This plot includes the 4 cities that have AR $\geq .5$ but appear to contain multiple normal distributions: Berlin, Santiago, Jakarta and Dublin.

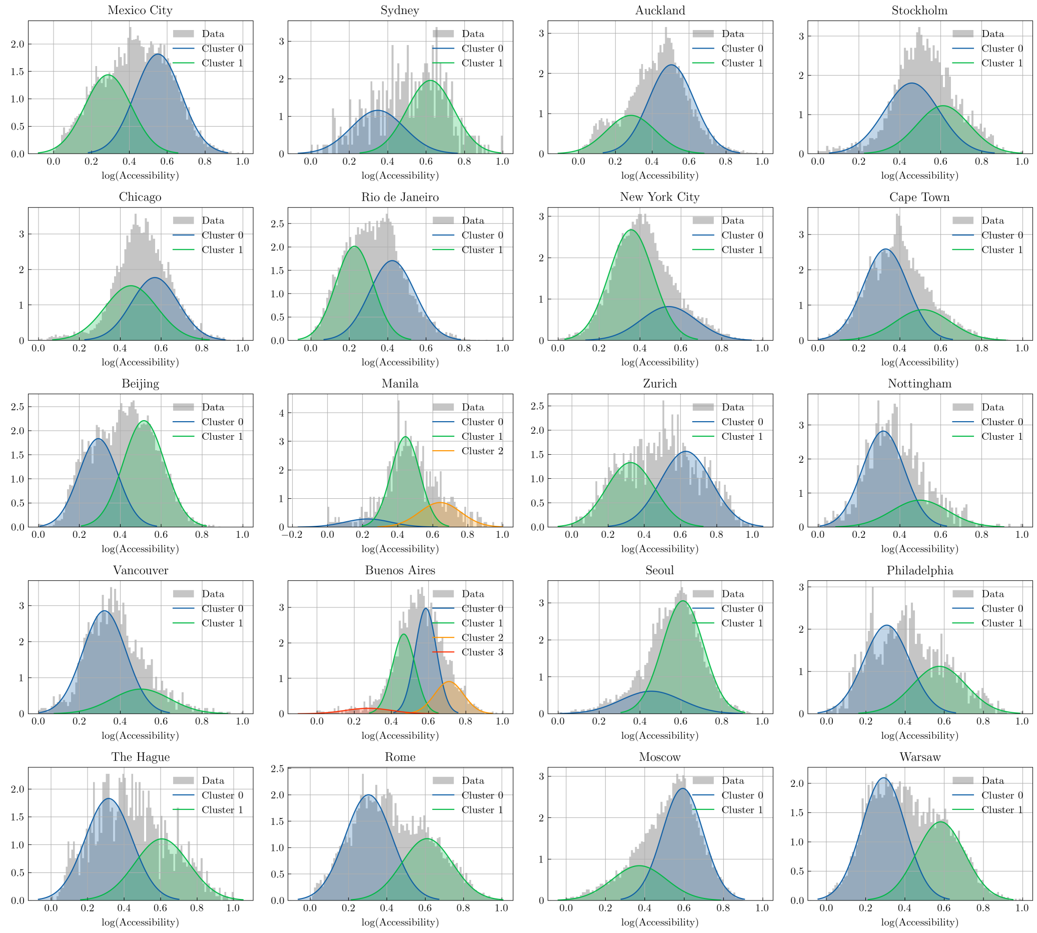


Supplementary Fig. 4: **part-1** Accessibility distributions of cities showing histograms and kernel density plots derived through Gaussian mixture modelling (GMM). Multiple normal distributions indicate different groups of accessibility that follow a normal distribution. We have not explored whether these groups are also socially or spatially correlated.

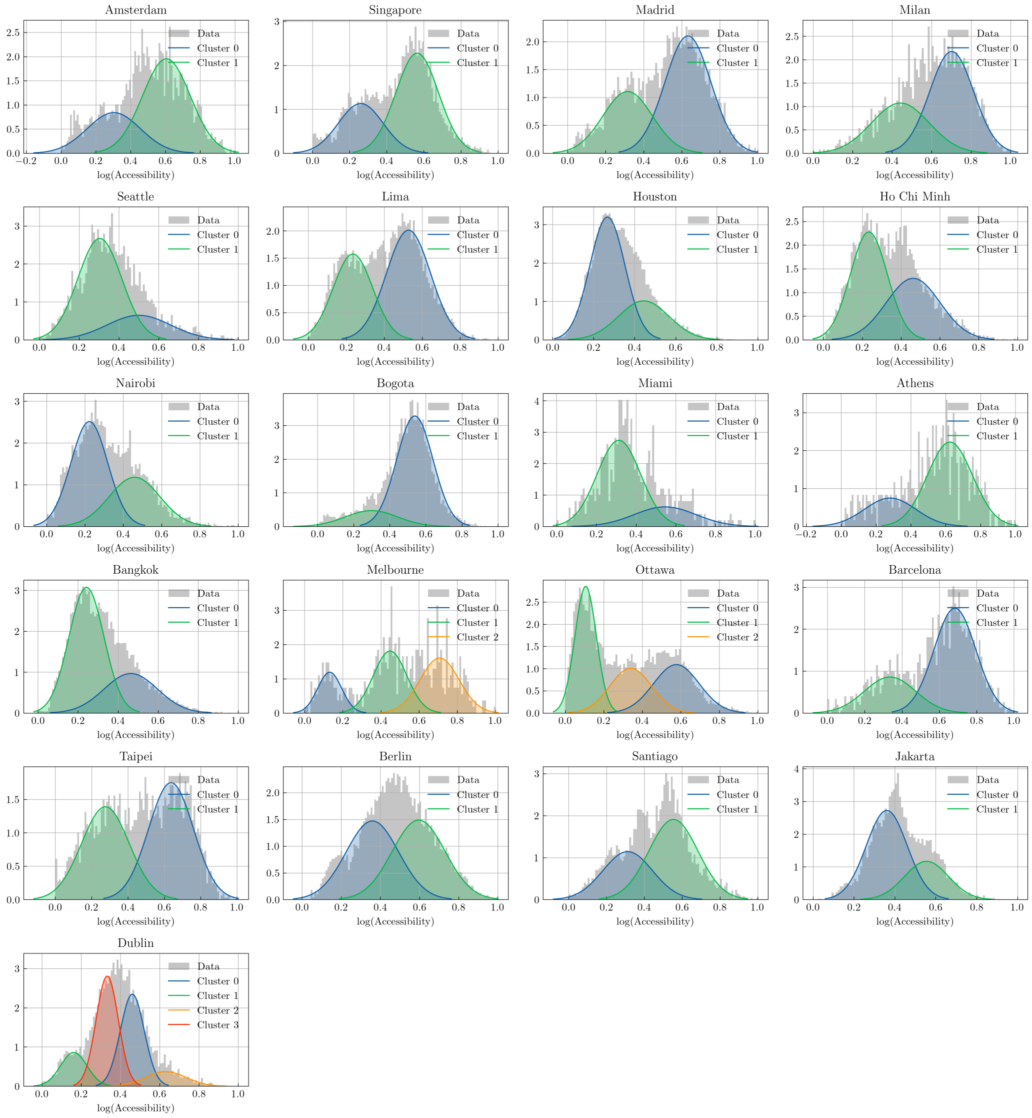


Supplementary Fig. 5: **part-2** Accessibility distributions of cities showing histograms and kernel density plots derived through Gaussian mixture modelling (GMM). Multiple normal distributions indicate different groups of accessibility that follow a normal distribution. We have not explored whether these groups are also socially or spatially correlated.

Supplementary Table 2: Acceptance Rate (AR) and *p*-values for the Shapiro-Wilk normality test on accessibility distributions of 54 cities in the data set. We run the test 100,000 times (trials) on different subsets of 250 observations (sampling without replacement) from the original sample. AR is calculated as a percentage of trials where the null hypothesis is accepted.

| **City** | **AR** | *p*-value | | | | | | |
|---|---|---|---|---|---|---|---|---|
| | | mean | std | min | 25% | 50% | 75% | max |
| Copenhagen | 0.9554 | 0.47 | 0.27 | 0.0 | 0.24 | 0.46 | 0.69 | 1.0 |
| Montreal | 0.8673 | 0.34 | 0.27 | 0.0 | 0.11 | 0.28 | 0.54 | 1.0 |
| Calgary | 0.8382 | 0.36 | 0.29 | 0.0 | 0.1 | 0.3 | 0.58 | 1.0 |
| Budapest | 0.8302 | 0.34 | 0.28 | 0.0 | 0.09 | 0.28 | 0.55 | 1.0 |
| Edmonton | 0.7968 | 0.32 | 0.28 | 0.0 | 0.07 | 0.24 | 0.51 | 1.0 |
| Berlin | 0.7769 | 0.19 | 0.18 | 0.0 | 0.06 | 0.14 | 0.28 | 0.97 |
| London | 0.7567 | 0.27 | 0.26 | 0.0 | 0.05 | 0.18 | 0.43 | 1.0 |
| Los Angeles | 0.7555 | 0.25 | 0.24 | 0.0 | 0.05 | 0.17 | 0.4 | 1.0 |
| Lisbon | 0.7499 | 0.24 | 0.24 | 0.0 | 0.05 | 0.15 | 0.36 | 1.0 |
| San Francisco | 0.6942 | 0.25 | 0.26 | 0.0 | 0.03 | 0.14 | 0.39 | 1.0 |
| Santiago | 0.6705 | 0.16 | 0.17 | 0.0 | 0.03 | 0.1 | 0.23 | 1.0 |
| Shanghai | 0.6654 | 0.14 | 0.15 | 0.0 | 0.03 | 0.09 | 0.21 | 0.93 |
| Edinburgh | 0.6226 | 0.14 | 0.16 | 0.0 | 0.03 | 0.08 | 0.19 | 0.97 |
| Jakarta | 0.6167 | 0.17 | 0.2 | 0.0 | 0.02 | 0.09 | 0.25 | 1.0 |
| Tokyo | 0.5854 | 0.2 | 0.25 | 0.0 | 0.01 | 0.09 | 0.32 | 1.0 |
| Istanbul | 0.5683 | 0.13 | 0.16 | 0.0 | 0.02 | 0.07 | 0.18 | 0.97 |
| Dublin | 0.5203 | 0.13 | 0.17 | 0.0 | 0.01 | 0.05 | 0.17 | 0.98 |
| Mexico City | 0.4998 | 0.1 | 0.13 | 0.0 | 0.01 | 0.05 | 0.14 | 0.98 |
| Sydney | 0.4738 | 0.09 | 0.12 | 0.0 | 0.01 | 0.05 | 0.12 | 0.92 |
| Auckland | 0.4443 | 0.1 | 0.14 | 0.0 | 0.01 | 0.04 | 0.12 | 0.94 |
| Stockholm | 0.4418 | 0.11 | 0.17 | 0.0 | 0.01 | 0.04 | 0.13 | 0.99 |
| Chicago | 0.3964 | 0.11 | 0.19 | 0.0 | 0.0 | 0.03 | 0.13 | 1.0 |
| Rio de Janeiro | 0.385 | 0.07 | 0.11 | 0.0 | 0.01 | 0.03 | 0.09 | 0.87 |
| New York City | 0.3765 | 0.1 | 0.18 | 0.0 | 0.0 | 0.02 | 0.12 | 0.99 |
| Cape Town | 0.3693 | 0.09 | 0.16 | 0.0 | 0.0 | 0.02 | 0.1 | 1.0 |
| Beijing | 0.3436 | 0.08 | 0.13 | 0.0 | 0.01 | 0.02 | 0.08 | 0.98 |
| Manila | 0.1977 | 0.04 | 0.08 | 0.0 | 0.0 | 0.01 | 0.04 | 0.85 |
| Zurich | 0.1928 | 0.03 | 0.06 | 0.0 | 0.0 | 0.01 | 0.04 | 0.79 |
| Nottingham | 0.1834 | 0.04 | 0.1 | 0.0 | 0.0 | 0.0 | 0.03 | 0.98 |
| Vancouver | 0.1773 | 0.04 | 0.11 | 0.0 | 0.0 | 0.0 | 0.02 | 0.95 |
| Buenos Aires | 0.149 | 0.04 | 0.13 | 0.0 | 0.0 | 0.0 | 0.01 | 1.0 |
| Seoul | 0.0968 | 0.02 | 0.08 | 0.0 | 0.0 | 0.0 | 0.01 | 0.91 |
| Philadelphia | 0.0879 | 0.02 | 0.04 | 0.0 | 0.0 | 0.0 | 0.01 | 0.66 |
| The Hague | 0.0759 | 0.02 | 0.03 | 0.0 | 0.0 | 0.0 | 0.01 | 0.5 |
| Rome | 0.0732 | 0.01 | 0.03 | 0.0 | 0.0 | 0.0 | 0.01 | 0.53 |
| Moscow | 0.0593 | 0.01 | 0.05 | 0.0 | 0.0 | 0.0 | 0.01 | 0.81 |
| Warsaw | 0.058 | 0.01 | 0.03 | 0.0 | 0.0 | 0.0 | 0.01 | 0.53 |
| Amsterdam | 0.0572 | 0.01 | 0.03 | 0.0 | 0.0 | 0.0 | 0.01 | 0.66 |
| Singapore | 0.0439 | 0.01 | 0.03 | 0.0 | 0.0 | 0.0 | 0.01 | 0.82 |
| Madrid | 0.0432 | 0.01 | 0.03 | 0.0 | 0.0 | 0.0 | 0.01 | 0.51 |
| Milan | 0.0326 | 0.01 | 0.03 | 0.0 | 0.0 | 0.0 | 0.0 | 0.6 |
| Seattle | 0.0282 | 0.01 | 0.03 | 0.0 | 0.0 | 0.0 | 0.0 | 0.64 |
| Lima | 0.0262 | 0.01 | 0.02 | 0.0 | 0.0 | 0.0 | 0.0 | 0.43 |
| Houston | 0.0217 | 0.0 | 0.03 | 0.0 | 0.0 | 0.0 | 0.0 | 0.98 |
| Ho Chi Minh | 0.0052 | 0.0 | 0.01 | 0.0 | 0.0 | 0.0 | 0.0 | 0.48 |
| Nairobi | 0.0048 | 0.0 | 0.01 | 0.0 | 0.0 | 0.0 | 0.0 | 0.19 |
| Bogota | 0.0016 | 0.0 | 0.01 | 0.0 | 0.0 | 0.0 | 0.0 | 0.26 |
| Miami | 0.0013 | 0.0 | 0.0 | 0.0 | 0.0 | 0.0 | 0.0 | 0.14 |
| Athens | 0.0005 | 0.0 | 0.0 | 0.0 | 0.0 | 0.0 | 0.0 | 0.11 |
| Bangkok | 0.0001 | 0.0 | 0.0 | 0.0 | 0.0 | 0.0 | 0.0 | 0.41 |
| Ottawa | 0.0 | 0.0 | 0.0 | 0.0 | 0.0 | 0.0 | 0.0 | 0.0 |
| Taipei | 0.0 | 0.0 | 0.0 | 0.0 | 0.0 | 0.0 | 0.0 | 0.04 |
| Barcelona | 0.0 | 0.0 | 0.0 | 0.0 | 0.0 | 0.0 | 0.0 | 0.02 |
| Melbourne | 0.0 | 0.0 | 0.0 | 0.0 | 0.0 | 0.0 | 0.0 | 0.0 |

# 2 Weights used to compute the accessibility score (A)

Supplementary Table 3: Weights used to compute the accessibility score (A) for each type of POIs collected.

| Category | Weight |
|---|---|
| Mobility | 0.2 |
| Active Living | 0.1 |
| Nightlife | 0.1 |
| Food Choices | 0.15 |
| Community Space | 0.1 |
| Education | 0.15 |
| Health and Wellbeing | 0.2 |

# 3 Demographic Categories used for Clustering

Supplementary Table 4: Socioeconomic variables used for consensus clustering using census information from Dissemination Areas (DA) in Canadian cities.

| **Socioeconomic Variables** |
|---|
| Population density per square kilometre |
| Average age of the population |
| Canadian citizens |
| Not Canadian citizens |
| Non-immigrants |
| Immigrants |
| First generation |
| Second generation |
| Third generation or more |
| Aboriginal identity |
| Non-Aboriginal identity |
| Total visible minority population |
| Number of persons in private households |
| Married |
| Not married and not living common law |
| Total couple families |
| Total lone-parent families by sex of parent |
| English only |
| French only |
| English and French |
| Neither English nor French |
| Average total income in 2015 among recipients ($) |
| Spending less than 30% of income on shelter costs |
| Spending 30% or more of income on shelter costs |
| Owner |
| Renter |
| Average value of dwellings ($) |
| Average monthly shelter costs for rented dwellings ($) |
| Average number of rooms per dwelling |
| No certificate, diploma or degree |
| Secondary (high) school diploma or equivalency certificate |
| Postsecondary certificate, diploma or degree |
| Employed |
| Unemployed |
| Management occupations |
| Business, finance and administration occupations |
| Natural and applied sciences and related occupations |
| Health occupations |
| Occupations in education, law and social, community and government services |
| Occupations in art, culture, recreation and sport |
| Sales and service occupations |
| Trades, transport and equipment operators and related occupations |
| Natural resources, agriculture and related production occupations |
| Occupations in manufacturing and utilities |

Supplementary Table 5: Socioeconomic variables used for consensus clustering using census information from Census Block Groups (CBG) in cities from USA.

| **Socioeconomic Variables** |
|---|
| Population |
| Age |
| White |
| Minority |
| Total households |
| Average household size |
| Married households |
| Nonfamily households |
| Median household income |
| Owner |
| Renter |
| Median gross rent |
| Total gross rent as percent of income |
| Less than 30 of income |
| More than 30 of income |
| Median gross rent as percent of income |
| Median n rooms |
| Less than high school |
| High school |
| Bachelors degree |
| Masters degree |
| Professional school degree |
| Doctorate degree |
| Employed |
| Unemployed |

# 4 Categories of Points of Interest

Supplementary Table 6: Points of Interest (POIs) classifier tags categorized into different classes of amenities.

| POI Classifier Tag | Categories of Amenities | | | | | | |
|---|---|---|---|---|---|---|---|
| | Mobility | Active Living | Entertainment | Food | Community | Education | Health and Wellbeing |
| transit_stop | X | | | | | | |
| bus_station | X | | | | | | |
| bus_stop | X | | | | | | |
| public_transport | X | | | | | | |
| bicycle_parking | | X | | | | | |
| gym | | X | | | | | |
| fitness_centre | | X | | | | | |
| sports_centre | | X | | | | | |
| park | | X | | | | | |
| pitch | | X | | | | | |
| playground | | X | | | | | |
| swimming_pool | | X | | | | | |
| garden | | X | | | | | |
| golf_course | | X | | | | | |
| sports_centre | | X | | | | | |
| ice_rink | | X | | | | | |
| dog_park | | X | | | | | |
| nature_reserve | | X | | | | | |
| fitness_centre | | X | | | | | |
| marina | | X | | | | | |
| recreation_ground | | X | | | | | |
| fitness_station | | X | | | | | |
| skate_park | | X | | | | | |
| pub | | | X | | | | |
| bar | | | X | | | | |
| theatre | | | X | | | | |
| cinema | | | X | | | | |
| nightclub | | | X | | | | |
| events_venue | | | X | | | | |
| restaurant | | | | X | | | |
| cafe | | | | X | | | |
| food_court | | | | X | | | |
| marketplace | | | | X | | | |
| community_centre | | | | X | | | |
| library | | | | | X | | |
| social_facility | | | | | X | | |
| social_centre | | | | | X | | |
| townhall | | | | | X | | |
| school | | | | | | X | |
| childcare | | | | | | X | |
| child_care | | | | | | X | |
| kindergarten | | | | | | X | |
| university | | | | | | X | |
| college | | | | | | | X |
| pharmacy | | | | | | | X |
| dentist | | | | | | | X |
| clinic | | | | | | | X |
| hospital | | | | | | | X |
| doctors | | | | | | | X |

# 5 Spatial representation of Clustered Demographics and Accessibility

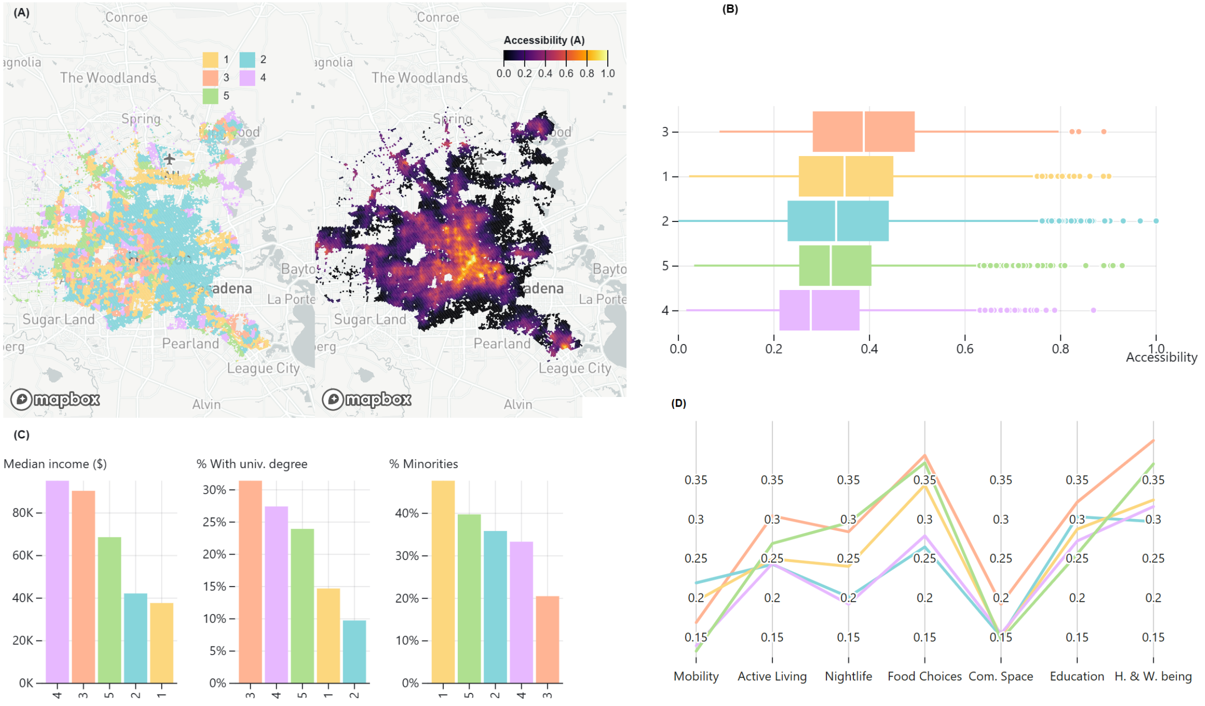


(a) Houston

Supplementary Fig. 6: (A) Spatial representation of the different clustered social groups for subset cities and the spatial distribution of accessibility for each city, where each spatial unit (an equal sized square of 0.0625 $km^2$) has its own accessibility score. (B) The statistical distribution of accessibility for each of the city's clustered social groups. (C) Statistical distribution of normalized key demographic attributes for each of the city's clustered social groups. (D) A parallel coordinates chart illustrating each social group's median accessibility scores disaggregated across amenity types.

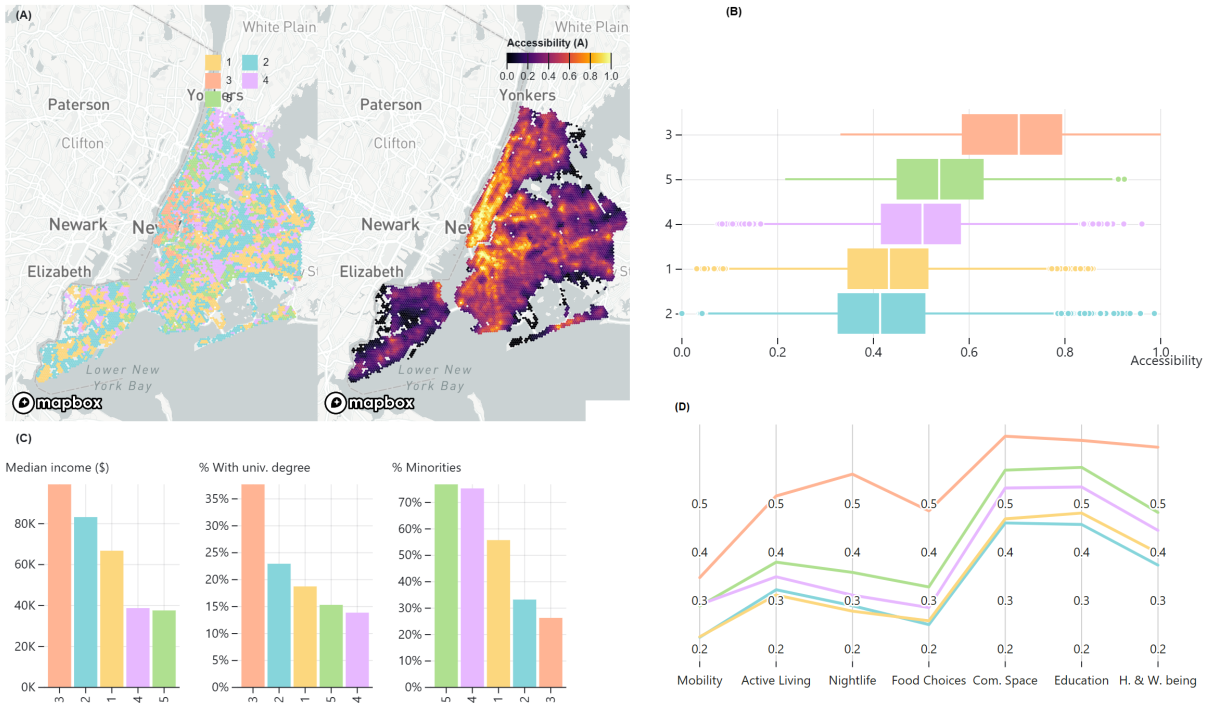


(b) New York City

Supplementary Fig. 6: (A) Spatial representation of the different clustered social groups for subset cities and the spatial distribution of accessibility for each city, where each spatial unit (an equal sized square of 0.0625 $km^2$) has its own accessibility score. (B) The statistical distribution of accessibility for each of the city's clustered social groups. (C) Statistical distribution of normalized key demographic attributes for each of the city's clustered social groups. (D) A parallel coordinates chart illustrating each social group's median accessibility scores disaggregated across amenity types. [continued.]

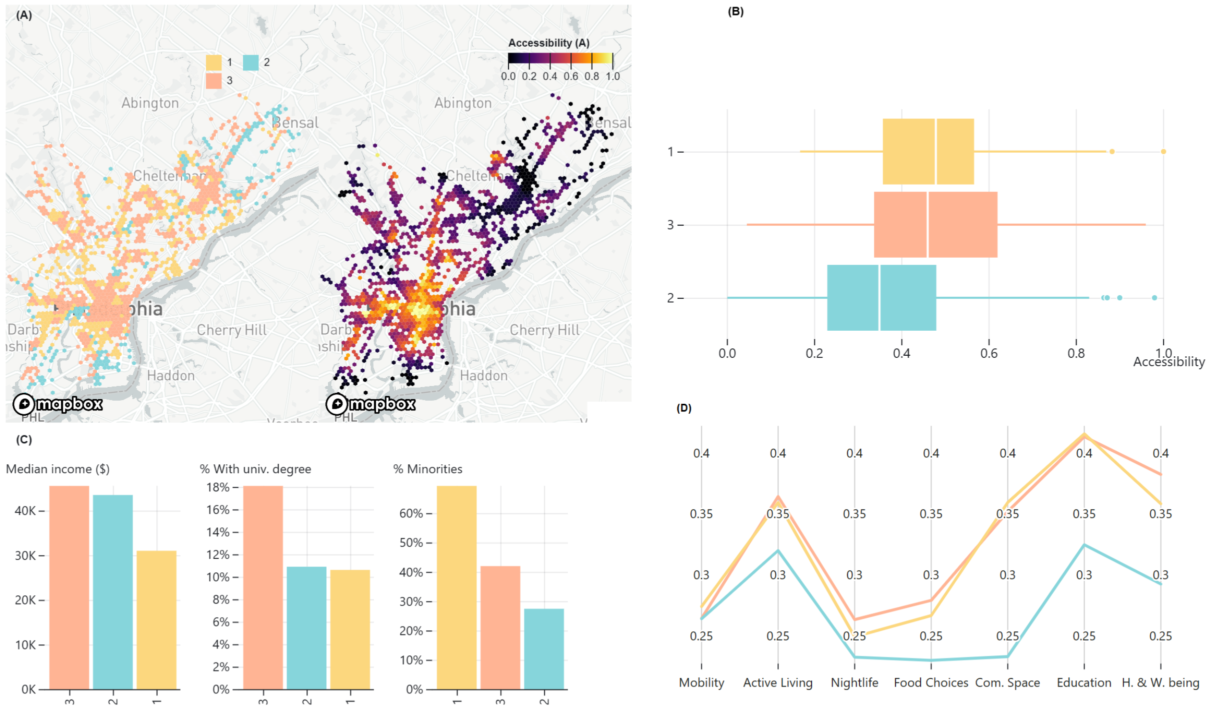


(c) Philadelphia

Supplementary Fig. 6: (A) Spatial representation of the different clustered social groups for subset cities and the spatial distribution of accessibility for each city, where each spatial unit (an equal sized square of 0.0625 $km^2$) has its own accessibility score. (B) The statistical distribution of accessibility for each of the city's clustered social groups. (C) Statistical distribution of normalized key demographic attributes for each of the city's clustered social groups. (D) A parallel coordinates chart illustrating each social group's median accessibility scores disaggregated across amenity types. [continued.]

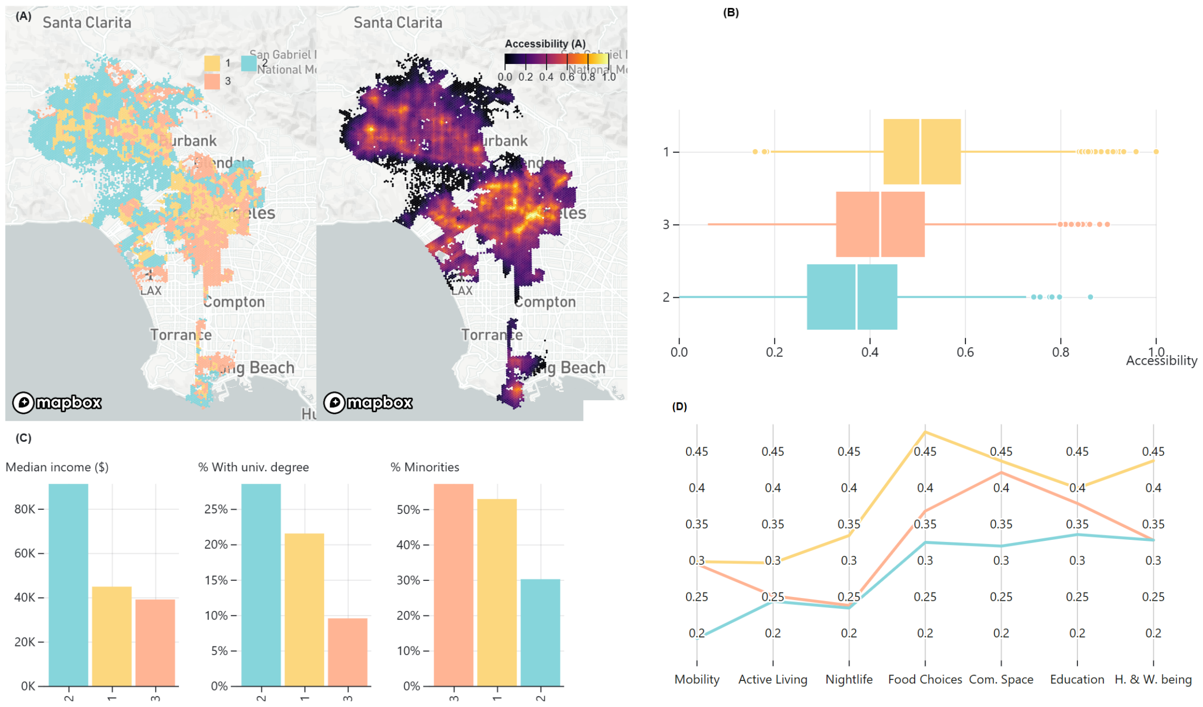


(d) Los Angeles

Supplementary Fig. 6: (A) Spatial representation of the different clustered social groups for subset cities and the spatial distribution of accessibility for each city, where each spatial unit (an equal sized square of 0.0625 $km^2$) has its own accessibility score. (B) The statistical distribution of accessibility for each of the city's clustered social groups. (C) Statistical distribution of normalized key demographic attributes for each of the city's clustered social groups. (D) A parallel coordinates chart illustrating each social group's median accessibility scores disaggregated across amenity types. [continued.]

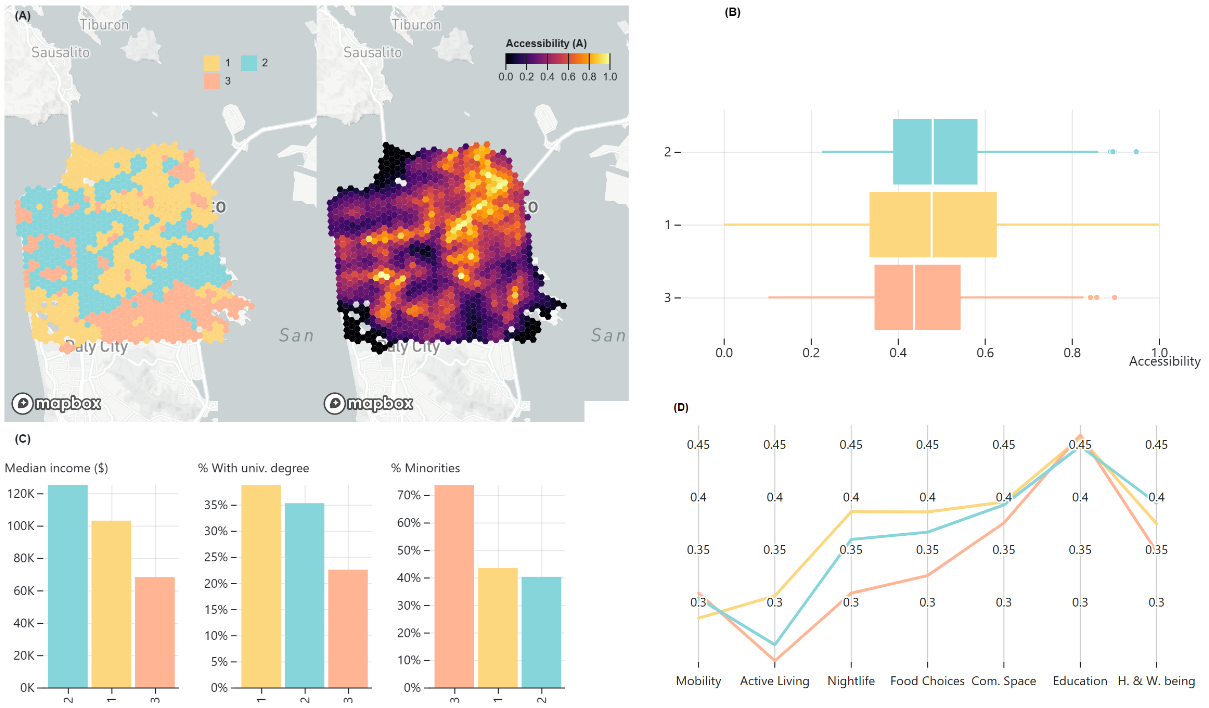


(e) San Francisco

Supplementary Fig. 6: (A) Spatial representation of the different clustered social groups for subset cities and the spatial distribution of accessibility for each city, where each spatial unit (an equal sized square of 0.0625 $km^2$) has its own accessibility score. (B) The statistical distribution of accessibility for each of the city's clustered social groups. (C) Statistical distribution of normalized key demographic attributes for each of the city's clustered social groups. (D) A parallel coordinates chart illustrating each social group's median accessibility scores disaggregated across amenity types. [continued.]

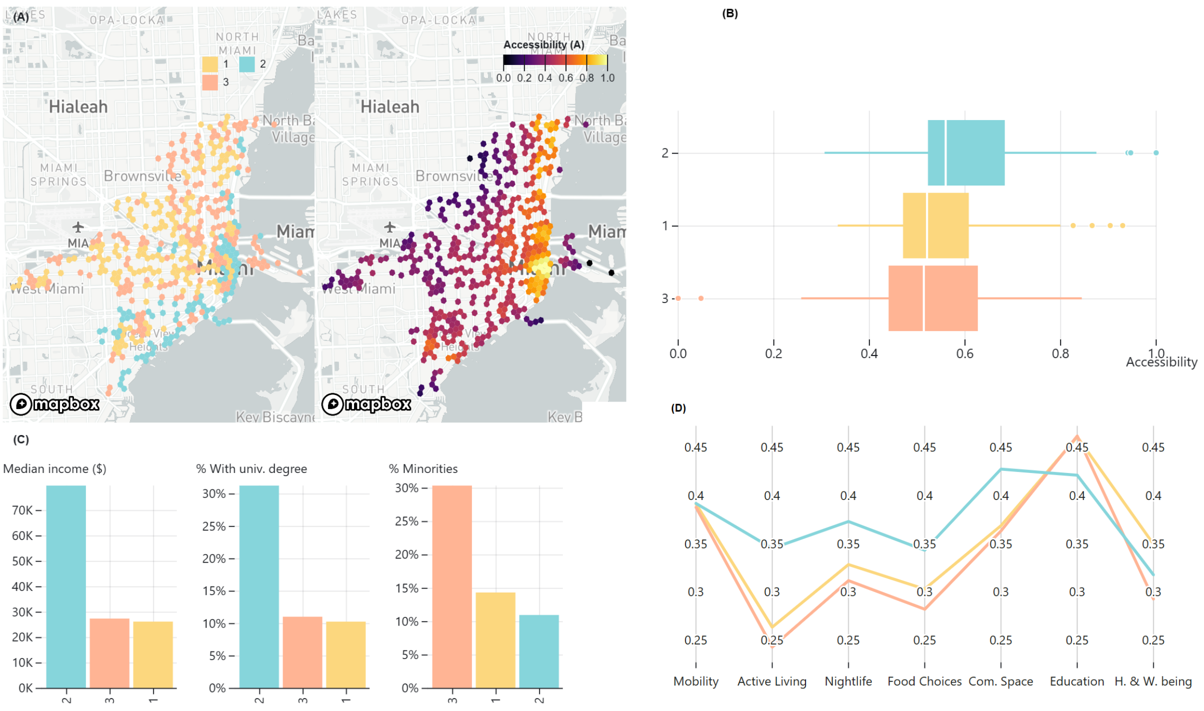


(f) Miami

Supplementary Fig. 6: (A) Spatial representation of the different clustered social groups for subset cities and the spatial distribution of accessibility for each city, where each spatial unit (an equal sized square of 0.0625 $km^2$) has its own accessibility score. (B) The statistical distribution of accessibility for each of the city's clustered social groups. (C) Statistical distribution of normalized key demographic attributes for each of the city's clustered social groups. (D) A parallel coordinates chart illustrating each social group's median accessibility scores disaggregated across amenity types. [continued.]

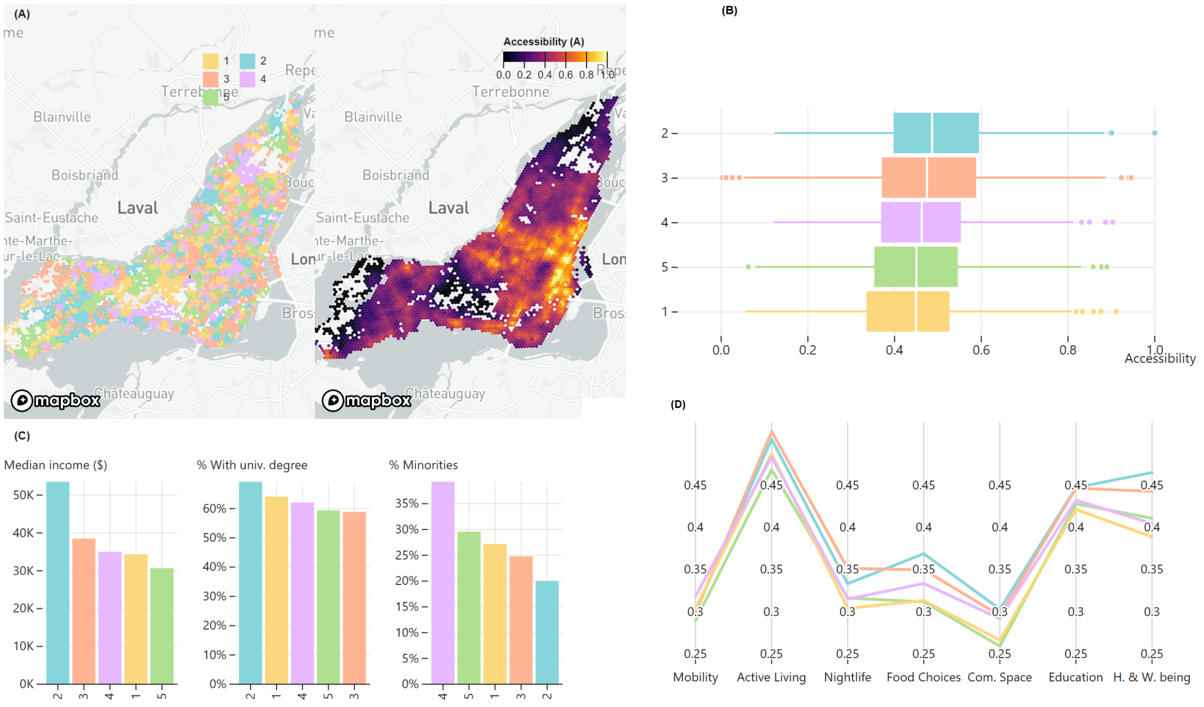


(g) Montreal

Supplementary Fig. 6: (A) Spatial representation of the different clustered social groups for subset cities and the spatial distribution of accessibility for each city, where each spatial unit (an equal sized square of 0.0625 $km^2$) has its own accessibility score. (B) The statistical distribution of accessibility for each of the city's clustered social groups. (C) Statistical distribution of normalized key demographic attributes for each of the city's clustered social groups. (D) A parallel coordinates chart illustrating each social group's median accessibility scores disaggregated across amenity types. [continued.]

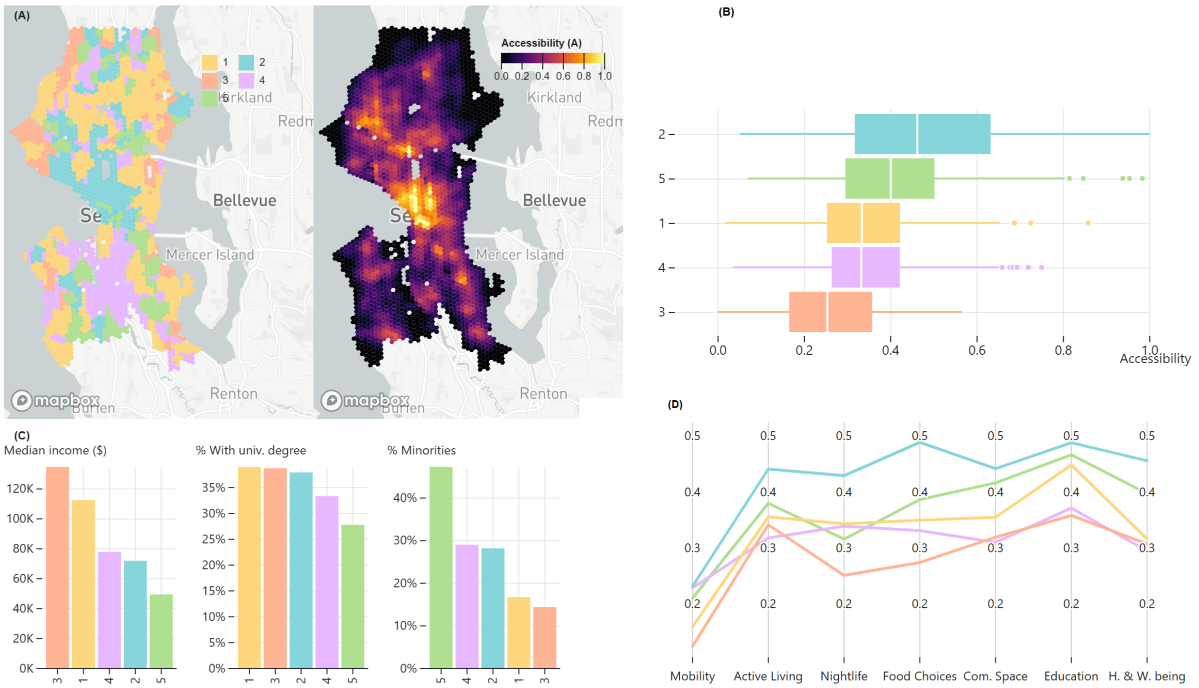


(h) Seattle

Supplementary Fig. 6: (A) Spatial representation of the different clustered social groups for subset cities and the spatial distribution of accessibility for each city, where each spatial unit (an equal sized square of 0.0625 $km^2$) has its own accessibility score. (B) The statistical distribution of accessibility for each of the city's clustered social groups. (C) Statistical distribution of normalized key demographic attributes for each of the city's clustered social groups. (D) A parallel coordinates chart illustrating each social group's median accessibility scores disaggregated across amenity types. [continued.]

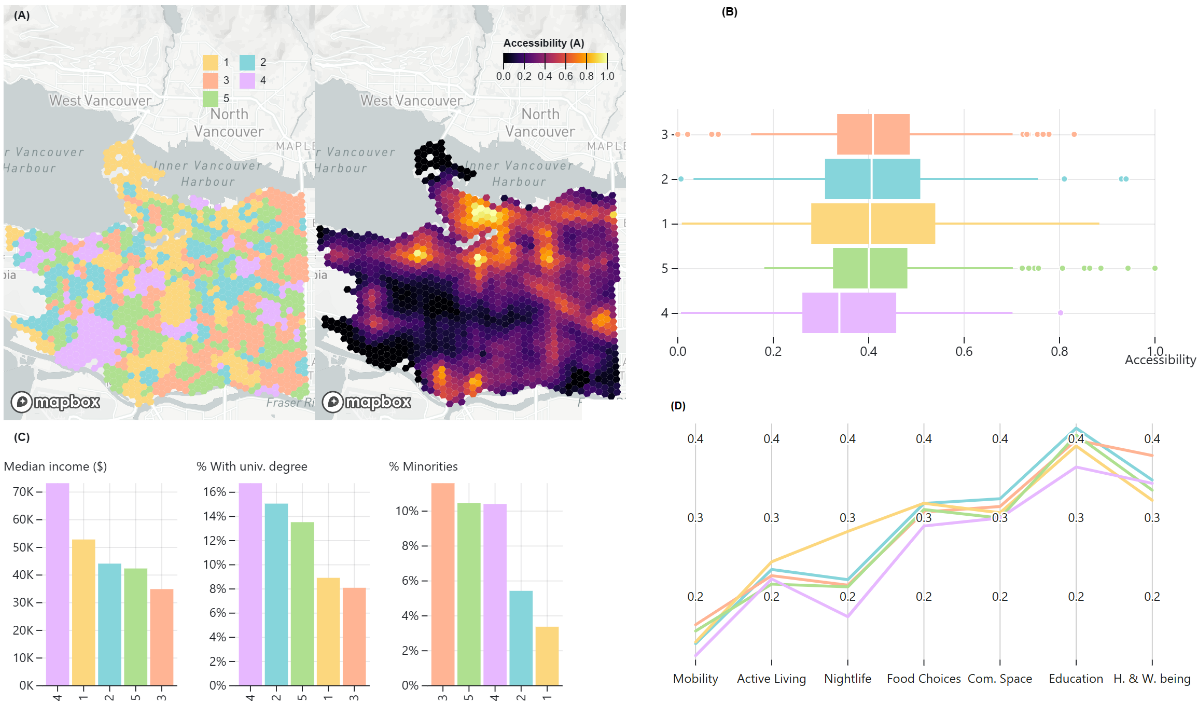


(i) Vancouver

Supplementary Fig. 6: (A) Spatial representation of the different clustered social groups for subset cities and the spatial distribution of accessibility for each city, where each spatial unit (an equal sized square of 0.0625 km$^2$) has its own accessibility score. (B) The statistical distribution of accessibility for each of the city's clustered social groups. (C) Statistical distribution of normalized key demographic attributes for each of the city's clustered social groups. (D) A parallel coordinates chart illustrating each social group's median accessibility scores disaggregated across amenity types. [continued.]

# References


1. N. M. Razali, Y. B. Wah, *et al.*, Power comparisons of shapiro-wilk, kolmogorov-smirnov, lilliefors and anderson-darling tests. *Journal of statistical modeling and analytics* **2**, 21–33 (2011).

2. G. Boeing, Osmnx: New methods for acquiring, constructing, analyzing, and visualizing complex street networks. *Computers, Environment and Urban Systems* **65**, 126–139 (2017).

3. E. Commission, Ghsl - global human settlement layer (2015).

4. A. P. Dempster, N. M. Laird, D. B. Rubin, Maximum Likelihood from Incomplete Data via the EM Algorithm. *Journal of the Royal Statistical Society. Series B (Methodological)* **39**, 1–38 (1977). Publisher: [Royal Statistical Society, Wiley].

5. T. Verma, M. Sirenko, I. Kornecki, S. Cunningham, N. A. Araújo, Extracting spatiotemporal commuting patterns from public transit data. *Journal of Urban Mobility* **1**, 100004 (2021).

6. D. Steinley, M. J. Brusco, Evaluating mixture modeling for clustering: recommendations and cautions. *Psychological Methods* **16**, 63–79 (2011).
